# Supplementary material for: Ontology Interoperability: A Comprehensive Framework for Industry-Scale Applications
Source: arXiv:2507.12311 source file (2026-12-02)
Supplement: Supplementary file 2 [file building-appendix.tex]

\chapter{Experiment Details for ODPs}

\section{Building Ontology Corpus}
\label{appendix: building ontology corpus}

\noindent This building ontology corpus is selected and evolved from~\citep{pritoni2021metadata}.

\begin{sidewaystable}
\caption{Building ontology corpus.}
\label{tab: building ontology corpus}
\begin{adjustbox}{width=1\columnwidth,center}
\begin{tabular}{|l|l|l|}                                                                                                           \hline
No. & Abbreviations & References                                                                                                \\ \hline
\#1   & DogOnt        & Dogont-ontology modeling for intelligent domotic environments~\citep{bonino2008dogont}                   \\ \hline
\#2   & ThinkHome     & Thinkhome energy efficiency in future smart homes~\citep{reinisch2011thinkhome}                          \\ \hline
\#3   & Basont        & Basont-a modular, adaptive building automation system ontology~\citep{ploennigs2012basont}               \\ \hline
\#4   & BOnSAI        & BOnSAI: a smart building ontology for ambient intelligence~\citep{stavropoulos2012bonsai}                \\ \hline
\#5   & SimModel      & SimModel: A domain data model for whole building energy simulation~\citep{o2011simmodel}                 \\ \hline
\#6   & Km4City       & Km4City Smart City API: an integrated support for mobility services~\citep{nesi2016km4city}              \\ \hline
\#7   & SAREF         & Created in close interaction with the industry: the smart appliances reference (SAREF)    
                      ontology~\citep{daniele2015created}                                                                        \\ \hline
\#8   & HTO           & An ontology design pattern for iot device tagging systems~\citep{charpenay2015ontology}                  \\ \hline
\#9   & Brick         & Brick: Towards a unified metadata schema for buildings~\citep{balaji2016brick}                           \\ \hline
\#10  & ifcOWL        & Converting the industry foundation classes to the web ontology language~\citep{schevers2005converting}   \\ \hline
\#11  & oneM2M        & Recent advancements in the Internet-of-Things related standards: A oneM2M perspective~\citep{park2016recent} 
                    \\ \hline
\#12  & SBMS          & Semantic BMS: Ontology for Analysis of Building Operation Efficiency~\citep{kuvcera2017semantic}         \\ \hline
\#13  & WoT           & Introducing Thing Descriptions and Interactions: An Ontology for the Web of Things~\citep{charpenay2016introducing}                     \\ \hline
\#14  & BACS          & Reusing Domain Ontologies in Linked Building Data: the Case of Building Automation and 
                    Control~\citep{terkaj2017reusing}     \\ \hline
\#15  & CRTLont       & Ontology-based modeling of control logic in building automation systems~\citep{schneider2017ontology}    \\ \hline
\#16  & RECore        & The realestatecore ontology~\citep{hammar2019realestatecore}                                             \\ \hline
\#17  & SAREF4BLDG    & Extending the SAREF ontology for building devices and topology~\citep{poveda2018extending}               \\ \hline
\#18  & SBOnto        & SBOnto: Ontology of smart building~\citep{vzavcek2017sbonto}                                             \\ \hline
\#19  & SEAS          & The SEAS Knowledge Model~\citep{lefranccois2017seas}                                                     \\ \hline
\#20  & SSN/SOSA      & Semantic Sensor Network Ontology~\citep{neuhaus2009semantic}                                             \\ \hline
\#21  & Onto-SB       & Onto-SB: human profile ontology for energy efficiency in smart building~\citep{degha2018onto}            \\ \hline
\#22  & OPM           & Ontology for Property Management~\citep{opm2018}                                                         \\ \hline
\#23  & BOT           & BOT: the building topology ontology of the W3C linked building data group~\citep{rasmussen2021bot}       \\ \hline
\#24  & EM-KPI        & Enhancing energy management at district and building levels via an EM-KPI ontology~\citep{yehongkpi}     \\ \hline
\#25  & OnCom         & An Ontology-Based Thermal Comfort Management System In Smart Buildings~\citep{orozco2019ontology}        \\ \hline
\#26  & Haystack      & Project Haystack Data Standards~\citep{john2020project}                                                  \\ \hline
\#27  & DB            & A Digital Buildings Ontology for Google's Real Estate~\citep{berkoben2020digital}                        \\ \hline
\#28  & OP            & From obXML to the OP ontology: developing a semantic model for occupancy profile~\citep{chavez2020obxml} \\ \hline
\#29  & RESPONSE      & Integrating building and iot data in demand response solutions~\citep{esnaola2019integrating}            \\ \hline
\#30  & TUBES         & TUBES System Ontology: Digitalization of building service systems~\citep{pauen2021tubes}                 \\ \hline
\end{tabular}
\end{adjustbox}
\end{sidewaystable}

\section{Use Case Evaluation of Energy Audits}
\label{appendix: competency questions in energy audits}

\noindent{We used the OWL inferencing engine to execute the queries on our building sample. If the inferencing engine is not used, all the nested relationships should be specified in the SPARQL queries. For example, replacing \textit{rdf:type} with \textit{rdf:type/rdfs:subClassOf*}.}

\begin{sidewaystable}
\renewcommand\arraystretch{1.2}
\caption{Building ontology prefixes and namespaces.}
\label{tab: prefixes and namespaces}
\begin{center}
\begin{tabular}{|l|l|l|}
\hline
Ontologies                          & Prefixes              & Namespaces\\
\hline
\small Brick                        & \small brick          & \small \url{https://brickschema.org/schema/Brick#}\\
\hline
\multirow{4}{*}{\small RECore}      & \small core           & \small \url{https://w3id.org/rec/core#}\\
                                    & \small asset          & \small \url{https://w3id.org/rec/asset#} \\
                                    & \small device         & \small \url{https://w3id.org/rec/device#} \\
                                    & \small analytics      & \small \url{https://w3id.org/rec/analytics#} \\                                 
\hline
\multirow{3}{*}{\small Haystack}    & \small ph             & \small \url{https://project-haystack.org/def/ph/3.9.11#}\\
                                    & \small phIoT          & \small \url{https://project-haystack.org/def/phIoT/3.9.11#}\\
                                    & \small phScience      & \small \url{https://project-haystack.org/def/phScience/3.9.11#}\\
\hline
\multirow{3}{*}{\small DB}          & \small db             & \small \url{http://www.google.com/digitalbuildings/0.0.1#}\\
                                    & \small db\_hvac       & \small \url{http://www.google.com/digitalbuildings/0.0.1/hvac#} \\
                                    & \small db\_subfields  & \small \url{http://www.google.com/digitalbuildings/0.0.1/subfields#} \\
\hline
\end{tabular}
\end{center}
\end{sidewaystable}

\begin{sidewaystable}
\caption{Competency questions in the use case evaluation of energy audits.}
\label{tab: competency questions in energy audits}
\footnotesize
\begin{tabular}{|M{1.5cm}|m{10cm}|m{10cm}|}
\multicolumn{3}{p{21.5cm}}{(i) Competency Questions Related to Building Spaces:} \\
\multicolumn{3}{p{21.5cm}}{} \\
\multicolumn{3}{p{21.5cm}}{\#01: What is the primary use of the building? If multiple uses, what is the fraction of floor area for each use?} \\
\multicolumn{3}{p{21.5cm}}{}                                                                                  \\ \hline
Ontologies & SPARQL Queries & Query Evaluations                                                             \\ \hline
Brick  & \begin{lstlisting}
SELECT ?function
WHERE {
BLDG:Building_003 brick:buildingPrimaryFunction ?function.
}
\end{lstlisting} & Partially Answered \newline (Can answer the question ``What is the primary use of the building?'' and will return multiple results if the model has multiple uses. Cannot answer ``What is the fraction of floor area for each use?'' because the function is defined for the building, not other location types) \\ \hline
RECore  & \begin{lstlisting} 
SELECT ?function
WHERE {
BLDG:Building_003 core:premisesType ?function.
}\end{lstlisting}  & Partially Answered \newline (Can answer the question ``What is the primary use of the building?'' and will return multiple results if the model has multiple uses. Cannot answer ``What is the fraction of floor area for each use?'' because core:hasPremiseType can be used for administrative grouping of spaces, such as building components, but the definition of floor area is missing)  \\ \hline
Haystack  & \begin{lstlisting} 
SELECT ?function
WHERE {
BLDG:Building_003 phIoT:primaryFunction ?function.
}\end{lstlisting}  & Partially Answered \newline (Can answer the question ``What is the primary use of the building?'' and will return multiple results if the model has multiple uses. Cannot answer ``What is the fraction of floor area for each use?'' because the function is defined for the building, not other location types)   \\ \hline
DB  & N/A   & Unable to answer \newline (No definition of building function type)     \\ \hline
\end{tabular}
\end{sidewaystable}

\begin{sidewaystable}
\footnotesize
\begin{tabular}{|M{1.5cm}|m{10cm}|m{10cm}|}
\multicolumn{3}{p{21.5cm}}{} \\
\multicolumn{3}{p{21.5cm}}{\#02: What are the HVAC zones and their respective air-conditioned areas in the building?} \\
\multicolumn{3}{p{21.5cm}}{} \\ \hline
Ontologies & SPARQL Queries & Query Evaluations            \\ \hline
Brick  & \begin{lstlisting} 
SELECT ?HVACZone ?conditionedArea
WHERE {
?HVACZone rdf:type brick:HVAC_Zone.
BLDG:Building_003 brick:hasPart ?HVACZone.
?HVACZone brick:hasPart ?conditionedArea.
}
\end{lstlisting}  & Fully Answered \\ \hline
RECore  & \begin{lstlisting}
SELECT ?HVACZone ?conditionedArea
WHERE {
?HVACZone rdf:type core:HVACZone.
BLDG:Building_003 core:hasPart ?HVACZone.
?HVACZone core:hasPart ?conditionedArea.
}
\end{lstlisting} & Fully Answered \\ \hline
Haystack  & \begin{lstlisting}
SELECT ?HVACZone ?conditionedArea
WHERE {
?HVACZone rdf:type phIoT:hvac-zone-space.
?HVACZone phIoT:siteRef BLDG:Building_003.
?conditionedArea phIoT:spaceRef ?HVACZone.
}
\end{lstlisting} & Fully Answered  \\ \hline
DB  & \begin{lstlisting}
SELECT ?HVACZone ?conditionedArea
WHERE {
?HVACZone rdf:type db_hvac:Zone_hvac.
BLDG:Building_003 db:hasPhysicalLocation ?HVACZone.
?HVACZone db:hasPhysicalLocation ?conditionedArea.
}
\end{lstlisting} & Partially Answered \newline (Can be queried, but using the property \textit{db:hasPhysicalLocation} for HVAC zones is not appropriate) \\ \hline
\end{tabular}
\end{sidewaystable}

\begin{sidewaystable}
\footnotesize
\begin{tabular}{|M{1.5cm}|m{10cm}|m{10cm}|}
\multicolumn{3}{p{21.5cm}}{} \\
\multicolumn{3}{p{21.5cm}}{\#03: What are all the rooms and their floors in the building?} \\
\multicolumn{3}{p{21.5cm}}{} \\ \hline
Ontologies & SPARQL Queries & Query Evaluations            \\ \hline
Brick  & \begin{lstlisting} 
SELECT ?floor ?room
WHERE {
?floor rdf:type brick:Floor.
BLDG:Building_003 brick:hasPart+ ?floor.
OPTIONAL {
    ?floor brick:hasPart ?room.
    ?room rdf:type brick:Room.
    }
}
\end{lstlisting}  & Fully Answered \newline (Floor might be part of the building, but it might also be part of a wing that is part of the building. For this reason, we use the ``+'' property path quantifier to say that it is related by at least one step of this property)\\ \hline
RECore  & \begin{lstlisting} 
SELECT ?floor ?room
WHERE {
?floor rdf:type core:Level. 
BLDG:Building_003 core:hasPart+ ?floor.
OPTIONAL {
    ?floor core:hasPart ?room.
    ?room rdf:type core:Room.
    }
}
\end{lstlisting} & Fully Answered \newline (Floor might be part of the building, but it might also be part of a wing that is part of the building. For this reason, we use the ``+'' property path quantifier to say that it is related by at least one step of this property) \\ \hline
Haystack  & \begin{lstlisting}
SELECT ?floor ?room
WHERE {
?floor rdf:type phIoT:floor. 
?floor phIoT:siteRef BLDG:Building_003.
OPTIONAL {
    ?room phIoT:spaceRef ?floor.
    ?room rdf:type phIoT:room.
    }
}
\end{lstlisting} & Fully Answered  \\ \hline
DB  & \begin{lstlisting}
SELECT ?floor ?room
WHERE {
BLDG:Building_003 db:hasFloor ?floor.
OPTIONAL {
    ?floor db:hasRoom ?room.
    }
}
\end{lstlisting} & Partially Answered \newline (Floor might be part of the building, but it might also be part of a wing that is part of the building. As hasFloor is not a transitive property, only non-transitive information can be queried) \\ \hline
\end{tabular}
\end{sidewaystable}

\begin{sidewaystable}
\footnotesize
\begin{tabular}{|M{1.5cm}|m{10cm}|m{10cm}|}
\multicolumn{3}{p{21.5cm}}{} \\
\multicolumn{3}{p{21.5cm}}{\#04: What is the function type of each room?} \\ 
\multicolumn{3}{p{21.5cm}}{} \\ \hline
Ontologies & SPARQL Queries & Query Evaluations            \\ \hline
Brick  & \begin{lstlisting} 
SELECT ?room ?roomType
WHERE {
?room rdf:type brick:Room.
BLDG:Building_003 brick:hasPart+ ?room.
?room rdf:type ?roomType.
}
\end{lstlisting} & Fully Answered \\ \hline
RECore  & \begin{lstlisting} 
SELECT ?room ?roomType
WHERE {
?room rdf:type core:Room.
BLDG:Building_003 core:hasPart+ ?room.
?room rdf:type ?roomType.
}
\end{lstlisting} & Fully Answered \\ \hline
Haystack  & \begin{lstlisting}
SELECT ?room ?roomType
WHERE {
?room rdf:type phIoT:room.
?room phIoT:siteRef BLDG:Building_003.
?room rdf:type ?roomType.
}
\end{lstlisting} & Partially Answered \newline (It can be queried, but all rooms are of the same general type) \\ \hline
DB  & \begin{lstlisting}
SELECT ?room ?roomType
WHERE {
BLDG:Building_003 db:hasFloor ?floor.
?floor db:hasRoom ?room.
?room rdf:type ?roomType.
}
\end{lstlisting} & Partially Answered \newline (It can be queried, but all rooms are of the same general type) \\ \hline
\end{tabular}
\end{sidewaystable}

\begin{sidewaystable}
\footnotesize
\begin{tabular}{|M{1.5cm}|m{10cm}|m{10cm}|}
\multicolumn{3}{p{21.5cm}}{} \\
\multicolumn{3}{p{21.5cm}}{\#05: What is the occupancy of each room?} \\ 
\multicolumn{3}{p{21.5cm}}{} \\ \hline
Ontologies & SPARQL Queries & Query Evaluations            \\ \hline
Brick  & \begin{lstlisting} 
SELECT ?room ?occupancyStatus
WHERE {
?room rdf:type brick:Room.
BLDG:Building_003 brick:hasPart+ ?room.
?room brick:hasPoint ?occupancyStatus. 
?occupancyStatus rdf:type brick:Occupancy_Status.
}
\end{lstlisting} & Fully Answered \\ \hline
RECore & \begin{lstlisting} 
SELECT ?room ?occupancyStatus
WHERE {
?room rdf:type core:Room.
BLDG:Building_003 core:hasPart+ ?room.
?room core:hasCapability ?occupancyStatus. 
?occupancyStatus rdf:type device:OccupancyState.
}
\end{lstlisting} & Fully Answered \\ \hline
Haystack         & \begin{lstlisting}
SELECT ?room ?occupancyStatus
WHERE {
?room rdf:type phIoT:room.
?room phIoT:siteRef BLDG:Building_003.
?occupancyStatus phIoT:spaceRef ?room. 
?occupancyStatus rdf:type phIoT:occupied.
}
\end{lstlisting}  & Fully Answered \\ \hline
DB  & N/A & Unable to Answer \newline (Although DB has db\_subfields:Occupancy to define the status of being occupied, there is no appropriate property that can be found to link db\_subfields:Room and db\_subfields:Occupancy) \\ \hline
\end{tabular}
\end{sidewaystable}

\begin{sidewaystable}
\footnotesize
\begin{tabular}{|M{1.5cm}|m{10cm}|m{10cm}|}
\multicolumn{3}{p{21.5cm}}{} \\
\multicolumn{3}{p{21.5cm}}{(ii) Competency Questions Related to Building Equipment and Systems:} \\
\multicolumn{3}{p{21.5cm}}{} \\
\multicolumn{3}{p{21.5cm}}{\#06: What are the pieces of equipment and systems of equipment in the building?} \\ 
\multicolumn{3}{p{21.5cm}}{} \\ \hline
Ontologies & SPARQL Queries & Query Evaluations               \\ \hline
Brick  & \begin{lstlisting}
SELECT ?equipment ?system 
WHERE {
{?equipment rdf:type brick:Equipment.}
UNION
{?system rdf:type brick:System.}
}
\end{lstlisting} & Fully Answered \\ \hline
RECore  & \begin{lstlisting}
SELECT ?equipment ?system
WHERE {
{?equipment rdf:type asset:Equipment.}
UNION
{?system rdf:type asset:System.}
}
\end{lstlisting} & Fully Answered \\ \hline
Haystack  & \begin{lstlisting}
SELECT ?equipment
WHERE {
?equipment rdf:type phIoT:equip. 
}
\end{lstlisting} & Partially Answered \newline (The definition of systems of equipment is not fully implemented in the ontology at the time of writing) \\ \hline
DB  & \begin{lstlisting}
SELECT ?equipment
WHERE {
?equipment rdf:type db:Equipment. 
}
\end{lstlisting} & Partially Answered \newline (No definition of systems of equipment) \\ \hline
\end{tabular}
\end{sidewaystable}

\begin{sidewaystable}
\footnotesize
\begin{tabular}{|M{1.5cm}|m{10cm}|m{10cm}|}
\multicolumn{3}{p{21.5cm}}{} \\
\multicolumn{3}{p{21.5cm}}{\#07: What are the properties (e.g., type, physical location, and functional area) of each piece of HVAC equipment?} \\
\multicolumn{3}{p{21.5cm}}{} \\ \hline
Ontologies & SPARQL Queries & Query Evaluations               \\ \hline
Brick  & \begin{lstlisting}
SELECT ?equipment ?type ?physicalLocation ?functionalArea
WHERE {
?equipment rdf:type brick:HVAC_Equipment.
?equipment rdf:type ?type.
?equipment brick:hasLocation ?physicalLocation.
?equipment brick:feedsAir+ ?functionalArea.
}
\end{lstlisting} & Fully Answered \\ \hline
RECore  & \begin{lstlisting}
SELECT ?equipment ?type ?physicalLocation ?functionalArea
WHERE {
?equipment rdf:type asset:HVACEquipment. 
?equipment rdf:type ?type.
?equipment core:locatedIn ?physicalLocation.
?equipment asset:feeds+ ?functionalArea.
}
\end{lstlisting} & Fully Answered \\ \hline
Haystack  & \begin{lstlisting}
SELECT ?equipment ?type ?physicalLocation ?functionalArea
WHERE {
?equipment rdf:type phIoT:airHandlingEquip. 
?equipment rdf:type ?type.
?equipment phIoT:spaceRef ?physicalLocation.
?functionalArea phIoT:airRef+ ?equipment.
}
\end{lstlisting} & Fully Answered \\ \hline
DB  & \begin{lstlisting}
SELECT ?equipment ?type ?physicalLocation
WHERE {
?equipment rdf:type db:Equipment. 
?equipment rdf:type ?type.
?equipment db:hasPhysicalLocation ?physicalLocation.
}
\end{lstlisting} & Partially Answered \newline (No appropriate property can be found to link db:Equipment and its functional areas)   \\ \hline
\end{tabular}
\end{sidewaystable}

\begin{sidewaystable}
\footnotesize
\begin{tabular}{|M{1.5cm}|m{9cm}|m{6.5cm}|}
\multicolumn{3}{p{21.5cm}}{} \\
\multicolumn{3}{p{21.5cm}}{\#08: What are the components of each piece of HVAC equipment and their structural relations?} \\ 
\multicolumn{3}{p{21.5cm}}{} \\ \hline
Ontologies & SPARQL Queries & Query Evaluations               \\ \hline
Brick  & \begin{lstlisting}
SELECT ?equipment ?component ?feedsAirComponent
WHERE {
?equipment rdf:type brick:HVAC_Equipment.
?equipment brick:hasPart+ ?component.
OPTIONAL {
    ?component brick:feedsAir ?feedsAirComponent. 
    }
}
\end{lstlisting} & Fully Answered \\ \hline
RECore  & \begin{lstlisting}
SELECT ?equipment ?component ?feedsAirComponent
WHERE {
?equipment rdf:type asset:HVACEquipment.
?equipment core:hasPart+ ?component.
OPTIONAL {
    ?component asset:feeds ?feedsAirComponent. 
    }
}
\end{lstlisting} & Fully Answered \\ \hline
Haystack  & \begin{lstlisting}
SELECT ?equipment ?component ?feedsAirComponent
WHERE {
?equipment rdf:type phIoT:airHandlingEquip.
?component phIoT:equipRef+ ?equipment.
OPTIONAL {
    ?feedsAirComponent phIoT:airRef ?component.
    }
}
\end{lstlisting} & Fully Answered \\ \hline
DB  & N/A & Unable to Answer \newline (The connection properties hasPart and feeds are not fully implemented in the ontology at the time of writing)   \\ \hline
\end{tabular}
\end{sidewaystable}

\begin{sidewaystable}
\footnotesize
\begin{tabular}{|M{1.5cm}|m{10cm}|m{10cm}|}
\multicolumn{3}{p{21.5cm}}{} \\
\multicolumn{3}{p{21.5cm}}{\#09: What is the energy use broken down by resource using the energy?} \\ 
\multicolumn{3}{p{21.5cm}}{} \\ \hline
Ontologies & SPARQL Queries & Query Evaluations               \\ \hline
Brick  & \begin{lstlisting}
SELECT ?equipment ?substance ?timeseries
WHERE {
?equipment rdf:type brick:Equipment.
?equipment brick:hasInputSubstance ?substance.
?substance rdf:type brick:Substance.
?equipment brick:hasPoint ?point.
?point rdf:type brick:Energy_Sensor.
?point brick:timeseries ?timeseries.
FILTER (?substance = brick:Chilled_Water)
}
\end{lstlisting} & Fully Answered \newline (Assuming the energy use is represented as a time series associated with the energy sensor. Substance must be specified in the query, e.g., brick:Chilled\_Water) \\ \hline
RECore  & \begin{lstlisting}
SELECT ?equipment ?substance ?timeseries
WHERE {
?equipment rdf:type asset:Equipment.
?equipment asset:substance ?substance.
?equipment core:hasCapability ?point.
?point rdf:type device:EnergySensor.
?point core:generatedObservation ?timeseries.
FILTER (?substance = "ChilledWater")
}
\end{lstlisting} & Partially Answered \newline (Assuming the energy use is represented as a time series associated with the energy sensor. Substance must be specified in the query, e.g., ``ChilledWater''. The property of asset:substance has no distinction between input and output)  \\ \hline
Haystack  & \begin{lstlisting}
SELECT ?equipment ?substance ?value ?dateTime
WHERE {
?equipment rdf:type phIoT:equip.
?equipment ph:inputs ?substance.
?substance rdf:type phScience:substance.
?point phIoT:equipRef ?equipment.
?point phIoT:pointFunction phIoT:sensor.
?point phIoT:curVal ?value.
?value ph:dateTime ?dateTime.
FILTER (?substance = phIoT:chilled-water)
}
\end{lstlisting} & Partially Answered \newline (Substance must be specified in the query, e.g., phIoT:chilled-water. Sensor type cannot be specified for Energy Sensor. Use the current point value with date and time as an alternative way to show the time-series data. Subscription to real-time sensor data is not achievable within the ontology, but may be possible by plugging in a SCRAM-based authentication protocol)  \\ \hline
DB  & N/A & Unable to Answer \newline (No properties related to  substance)  \\ \hline
\end{tabular}
\end{sidewaystable}

\begin{sidewaystable}
\footnotesize
\begin{tabular}{|M{1.5cm}|m{10cm}|m{10cm}|}
\multicolumn{3}{p{21.5cm}}{} \\
\multicolumn{3}{p{21.5cm}}{\#10: What is the energy use broken down by end-use?} \\ 
\multicolumn{3}{p{21.5cm}}{} \\ \hline
Ontologies & SPARQL Queries & Query Evaluations               \\ \hline
Brick  & \begin{lstlisting}
SELECT ?equipment ?type ?timeseries
WHERE {
?equipment rdf:type brick:Equipment.
?equipment rdf:type ?type.
?equipment brick:hasPoint ?point.
?point rdf:type brick:Energy_Sensor.
?point brick:timeseries ?timeseries.
FILTER (?type = brick:HVAC_Equipment)
}
\end{lstlisting} & Fully Answered \newline (Assuming the energy use is represented as a time series associated with energy sensor. End-use equipment must be specified in the query, e.g., brick:HVAC\_Equipment)  \\ \hline
RECore  & \begin{lstlisting}
SELECT ?equipment ?type ?timeseries
WHERE {
?equipment rdf:type asset:Equipment.
?equipment rdf:type ?type.
?equipment core:hasCapability ?point.
?point rdf:type device:EnergySensor.
?point core:generatedObservation ?timeseries.
FILTER (?type = asset:HVACEquipment)
}
\end{lstlisting} & Fully Answered \newline (Assuming the energy use is represented as a time series associated with energy sensor. End-use equipment must be specified in the query, e.g., asset:HVACEquipment)  \\ \hline
Haystack  & \begin{lstlisting}
SELECT ?equipment ?type ?value ?dateTime
WHERE {
?equipment rdf:type phIoT:equip.
?equipment rdf:type ?type.
?point phIoT:equipRef ?equipment.
?point phIoT:pointFunction phIoT:sensor.
?point phIoT:curVal ?value.
?value ph:dateTime ?dateTime.
FILTER (?type = phIoT:airHandlingEquip)
}
\end{lstlisting} & Partially Answered \newline (End-use equipment must be specified in the query, e.g., phIoT:airHandlingEquip. Sensor type cannot be specified for Energy Sensor. Use the current point value with date and time as an alternative way to show the time-series data. Subscription to real-time sensor data is not achievable within the ontology, but may be possible by plugging in a SCRAM-based authentication protocol)  \\ \hline
DB  & N/A & Unable to answer \newline (No classification of end-use)  \\ \hline
\end{tabular}
\end{sidewaystable}

\begin{sidewaystable}
\footnotesize
\begin{tabular}{|M{1.5cm}|m{10cm}|m{10cm}|}
\multicolumn{3}{p{21.5cm}}{} \\
\multicolumn{3}{p{21.5cm}}{\#11: What are the energy-generating pieces of equipment in the building?} \\
\multicolumn{3}{p{21.5cm}}{} \\ \hline
Ontologies & SPARQL Queries & Query Evaluations               \\ \hline
Brick  & \begin{lstlisting}
SELECT ?equipment ?type
WHERE {
{?equipment rdf:type brick:PV_Panel.}
UNION
{?equipment rdf:type brick:Solar_Thermal_Collector.}
?equipment rdf:type ?type.
}
\end{lstlisting} & Partially Answered \newline (Some classes can be found, but no clear classification. Each relevant class should be specified in the query, e.g., brick:PV\_Panel and brick:Solar\_Thermal\_Collector) \\ \hline
RECore  & \begin{lstlisting}
SELECT ?equipment ?type
WHERE {
?equipment rdf:type asset:Generator.
?equipment rdf:type ?type.
}
\end{lstlisting} & Fully Answered \\ \hline
Haystack  & N/A & Unable to Answer \newline (No definitions of energy-generating pieces of equipment)  \\ \hline
DB  & N/A & Unable to Answer \newline (No definitions of energy-generating pieces of equipment)   \\ \hline
\end{tabular}
\end{sidewaystable}

\begin{sidewaystable}
\footnotesize
\begin{tabular}{|M{1.5cm}|m{10cm}|m{10cm}|}
\multicolumn{3}{p{21.5cm}}{} \\
\multicolumn{3}{p{21.5cm}}{(iii) Competency Questions Related to Building Points and Measurements:} \\
\multicolumn{3}{p{21.5cm}}{} \\
\multicolumn{3}{p{21.5cm}}{\#12: What are the meters and meter types in the building?} \\
\multicolumn{3}{p{21.5cm}}{} \\ \hline
Ontologies & SPARQL Queries & Query Evaluations               \\ \hline
Brick  & \begin{lstlisting}
SELECT ?meter ?meterType
WHERE {
?meter rdf:type brick:Meter.
?meter rdf:type ?meterType.
}
\end{lstlisting} & Fully Answered \\ \hline
RECore  & \begin{lstlisting}
SELECT ?meter ?meterType
WHERE {
?meter rdf:type asset:Meter.
?meter rdf:type ?meterType.
}
\end{lstlisting} & Fully Answered \\ \hline
Haystack  & \begin{lstlisting}
SELECT ?meter ?meterType
WHERE {
?meter rdf:type phIoT:meter.
?meter rdf:type ?meterType.
}
\end{lstlisting} & Fully Answered  \\ \hline
DB  & N/A &  Unable to Answer \newline (No definition of meter)  \\ \hline
\end{tabular}
\end{sidewaystable}

\begin{sidewaystable}
\footnotesize
\begin{tabular}{|M{1.5cm}|m{10cm}|m{10cm}|}
\multicolumn{3}{p{21.5cm}}{} \\
\multicolumn{3}{p{21.5cm}}{\#13: What does each meter measure (i.e., substance and quantity)?} \\
\multicolumn{3}{p{21.5cm}}{} \\ \hline
Ontologies & SPARQL Queries & Query Evaluations               \\ \hline
Brick  & \begin{lstlisting}
SELECT ?meter ?substanceAndQuantitykind
WHERE {
?meter rdf:type brick:Meter.
?meter brick:measures ?substanceAndQuantitykind.
}
\end{lstlisting} & Partially Answered \newline (Properties of substance and quantity exist, but it is not possible to relate the substance measured to the quantity kind, unless it is assumed that each meter measures only one substance)  \\ \hline
RECore  & \begin{lstlisting}
SELECT ?meter ?substanceAndQuantitykind
WHERE {
?meter rdf:type asset:Meter.
?meter core:observes ?substanceAndQuantitykind.
}
\end{lstlisting} & Partially Answered \newline (Properties of substance and quantity exist, but it is not possible to relate the substance measured to the quantity kind, unless it is assumed that each meter measures only one substance) \\ \hline
Haystack  & \begin{lstlisting}
SELECT ?meter ?substance ?quantitykind
WHERE {
?meter rdf:type phIoT:meter.
?meter phIoT:pointSubject ?substance.
?meter phIoT:pointQuantity ?quantitykind.
}
\end{lstlisting} & Fully Answered  \\ \hline
DB  & N/A & Unable to Answer \newline (No definition of meter) \\ \hline
\end{tabular}
\end{sidewaystable}

\begin{sidewaystable}
\footnotesize
\begin{tabular}{|M{1.5cm}|m{10cm}|m{10cm}|}
\multicolumn{3}{p{21.5cm}}{} \\
\multicolumn{3}{p{21.5cm}}{\#14: What are the connections between meters and sub-meters?} \\
\multicolumn{3}{p{21.5cm}}{} \\ \hline
Ontologies & SPARQL Queries & Query Evaluations               \\ \hline
Brick  & \begin{lstlisting}
SELECT ?meter ?subMeter
WHERE {
?meter rdf:type brick:Meter.
?subMeter rdf:type brick:Meter.
?meter brick:feeds ?subMeter.
}
\end{lstlisting} & Partially Answered \newline (We adopt brick:feeds as an unofficial convention in our models: meter closest to utility point of connection ``feeds'' sub-meters) \\ \hline
RECore  & \begin{lstlisting}
SELECT ?meter ?subMeter
WHERE {
?meter rdf:type asset:Meter.
?subMeter rdf:type asset:Meter.
?meter core:feeds ?subMeter.
}
\end{lstlisting} & Partially Answered \newline (We adopt core:feeds as an unofficial convention in our models: meter closest to utility point of connection ``feeds'' sub-meters)  \\ \hline
Haystack  & \begin{lstlisting}
SELECT ?meter ?subMeter
WHERE {
?meter rdf:type phIoT:meter.
?subMeter rdf:type phIoT:meter.
?subMeter phIoT:submeterOf ?meter.
}
\end{lstlisting} & Fully Answered  \\ \hline
DB  & N/A & Unable to Answer \newline (No definition of meter)  \\ \hline
\end{tabular}
\end{sidewaystable}

\begin{sidewaystable}
\footnotesize
\begin{tabular}{|M{1.5cm}|m{10cm}|m{10cm}|}
\multicolumn{3}{p{21.5cm}}{} \\
\multicolumn{3}{p{21.5cm}}{\#15: What are the operating parameters of each piece of equipment (e.g., setpoints and schedules)?} \\
\multicolumn{3}{p{21.5cm}}{} \\ \hline
Ontologies & SPARQL Queries & Query Evaluations               \\ \hline
Brick  & \begin{lstlisting}
SELECT ?equipment ?parameter
WHERE {
?equipment rdf:type brick:Equipment.
?equipment brick:hasPoint ?parameter.
?parameter rdf:type brick:Point.
}
\end{lstlisting} & Fully Answered \\ \hline
RECore  & \begin{lstlisting}
SELECT ?equipment ?parameter
WHERE {
?equipment rdf:type asset:Equipment.
?equipment core:hasCapability ?parameter.
?parameter rdf:type core:Capability.
}
\end{lstlisting} & Fully Answered  \\ \hline
Haystack  & \begin{lstlisting}
SELECT ?equipment ?parameter
WHERE {
?equipment rdf:type phIoT:equip.
?point phIoT:equipRef ?equipment.
?point rdf:type phIoT:point.
?point phIoT:pointFunction ?parameter.
}
\end{lstlisting} & Fully Answered  \\ \hline
DB  & N/A & Unable to answer \newline (No appropriate property can be found to link db:Equipment and its operating parameters)  \\ \hline
\end{tabular}
\end{sidewaystable}

\begin{sidewaystable}
\footnotesize
\begin{tabular}{|M{1.5cm}|m{10cm}|m{10cm}|}
\multicolumn{3}{p{21.5cm}}{} \\
\multicolumn{3}{p{21.5cm}}{\#16: What are the time series for each meter?} \\
\multicolumn{3}{p{21.5cm}}{} \\ \hline
Ontologies & SPARQL Queries & Query Evaluations               \\ \hline
Brick  & \begin{lstlisting}
SELECT ?meter ?timeseriesId
WHERE {
?meter rdf:type brick:Meter.
?meter brick:timeseries ?timeseries.
?timeseries brick:hasTimeseriesId ?timeseriesId.
}
\end{lstlisting} & Fully Answered \\ \hline
RECore  & \begin{lstlisting}
SELECT ?meter ?timeseriesId
WHERE {
?meter rdf:type asset:Meter.
?meter core:generatedObservation ?timeseries.
?timeseriesId analytics:seriesMembers ?timeseries.
}
\end{lstlisting} & Fully Answered  \\ \hline
Haystack  & \begin{lstlisting}
SELECT ?meter ?value ?dateTime
WHERE {
?meter rdf:type phIoT:meter.
?meter phIoT:curVal ?value.
?value ph:dateTime ?dateTime.
}
\end{lstlisting} & Particularly Answered \newline(Use the current point value with date and time as an alternative way to show the time-series data. Subscription to real-time sensor data is not achievable within the ontology, but may be possible by plugging in a SCRAM-based authentication protocol)  \\ \hline
DB  & N/A & Unable to Answer \newline (No definition of meter) \\ \hline
\end{tabular}
\end{sidewaystable}

\paragraph*{Publication Statement}

Most of the work presented in this chapter has been published as~\bibentry{qiang2023systematic}.
